# Supplementary material for: DEVIAS: Learning Disentangled Video Representations of Action and Scene
Source: arXiv:2312.00826 source file (2024-09-06)
Supplement: Supplementary file 1 [file slot_assignment.tex]

\begin{table}[h]
\centering

\caption{\textbf{Slot assignments in action recognition and scene recognition on UCF-101.}  We present the slot selection results of DEVIAS on UCF-101 dataset. We employ 4550 SCUBA-Places videos for action recognition and 3783 Scene-Only videos for scene recognition. The numbers inside the table mean the frequency of being selected for each column's slot.}

% \resizebox{0.9\columnwidth}{!}{
\fontsize{7.5pt}{9.5pt}\selectfont
\begin{tabular}{cc c c c c c}
\toprule
 && \multicolumn{2}{c}{Action} && \multicolumn{2}{c}{Scene} \\
\cline{3-4} \cline{6-7}
 && In-Context & Out-of-Context && In-Context & Out-of-Context \\
 && UCF-101 & SCUBA-Places && UCF-101 & Scene-Only \\

\midrule
\multirow{2}{*}{Slot 1} & Action Slot & - & 4550 && - & 3783 \\
 & Scene Slot & - & 0 && - & 0 \\

\midrule

\multirow{2}{*}{Slot 2} & Action Slot & - & 0 && - & 0 \\
 & Scene Slot & - & 4550 && - & 3783 \\

\bottomrule
\end{tabular}
\label{tab:slot_assign}
\end{table}

%%%%%%%%%%%%%%%%%%%%

\begin{table}[h]
\centering

\caption{\geo{Layout ?}}

% \resizebox{0.9\columnwidth}{!}{
\fontsize{7.5pt}{9.5pt}\selectfont
\begin{tabular}{ c | c | c | c }
\toprule
Dataset && Action Slot & Scene Slot \\

\midrule

\multirow{2}{*}{SCUBA-Places} & Slot 1 & 4550 & 0 \\
\cmidrule{2-4}
 & Slot 2 & 0 & 4550 \\

\midrule

\multirow{2}{*}{Scene-Only} & Slot 1 & 3783 & 0 \\
\cmidrule{2-4}
 & Slot 2 & 0 & 3783 \\

\bottomrule
\end{tabular}
\label{tab:slot_assign}
\end{table}

%%%%%%%%%%%%%%%%%%%%
\begin{table}[h]
\centering

\caption{\geo{Layout ?}}
    \mpage{0.48}{(a) Out-of-Context}
    \hfill
    \mpage{0.48}{(b) In-Context}
    \\
    \mpage{0.48}{
    % \resizebox{0.9\columnwidth}{!}{
    \fontsize{7.5pt}{9.5pt}\selectfont
    \begin{tabular}{c c  c  c  c }
    \toprule
    Dataset & Target && Action Slot & Scene Slot \\
    
    \midrule
    
    \multirow{2}{*}{SCUBA-Places} & \multirow{2}{*}{Action} & Slot 1 & 4550 & 0 \\
    \cmidrule{3-5}
     && Slot 2 & 0 & 4550 \\
    
    \midrule
    
    \multirow{2}{*}{Scene-Only} & \multirow{2}{*}{Scene} & Slot 1 & 3783 & 0 \\
    \cmidrule{3-5}
     && Slot 2 & 0 & 3783 \\
    
    \bottomrule
    \end{tabular}
    }
    \hfill
    \mpage{0.48}{
    % \resizebox{0.9\columnwidth}{!}{
    \fontsize{7.5pt}{9.5pt}\selectfont
    \begin{tabular}{c c  c  c  c }
    \toprule
    Dataset & Target && Action Slot & Scene Slot \\
    
    \midrule
    
    \multirow{4}{*}{UCF-101} & \multirow{2}{*}{Action} & Slot 1 & - & 0 \\
    \cmidrule{3-5}
     && Slot 2 & 0 & - \\
    
    \cmidrule{2-5}
    
     & \multirow{2}{*}{Scene} & Slot 1 & - & 0 \\
    \cmidrule{3-5}
     && Slot 2 & 0 & - \\
    
    \bottomrule
    \end{tabular}
    }
    
\label{tab:slot_assign}
\end{table}

%%%%%%%%%%%%%%%%%%%%
\begin{table}[h]
\centering

\caption{\geo{Layout ?}}

% \resizebox{0.9\columnwidth}{!}{
\fontsize{7.5pt}{9.5pt}\selectfont
\begin{tabular}{ c  c  c  c }
\toprule
Dataset && Action Slot & Scene Slot \\

\midrule

\multirow{2}{*}{SCUBA-Places} & Slot 1 & 4550 & 0 \\
 & \cellcolor{gray!30}Slot 2 & \cellcolor{gray!30}0 & \cellcolor{gray!30}4550 \\

\midrule

\multirow{2}{*}{Scene-Only} & Slot 1 & 3783 & 0 \\
 & \cellcolor{gray!30}Slot 2 & \cellcolor{gray!30}0 & \cellcolor{gray!30}3783 \\

\bottomrule
\end{tabular}
\label{tab:slot_assign}
\end{table}
