# Supplementary material for: DEVIAS: Learning Disentangled Video Representations of Action and Scene
Source: arXiv:2312.00826 source file (2024-09-06)
Supplement: Supplementary file 4 [file baseline_noaug.tex]

\begin{table}[t]
\centering
\caption{\tb{Hyperparameters used for training the disentangling baselines on each dataset.}}
\vspace{1em}
\resizebox{\columnwidth}{!}{
\begin{tabular}{lcc}
    
% \shline
\toprule
Config & UCF-101 & Kinetics-400 \\
% \shline
\midrule
Optimizer &   AdamW~\cite{adamw}& AdamW \\
Base learning rate &   5e-4 &5e-4 \\
Weight decay &   0.05 &0.05  \\
Optimizer momentum &   {$\beta_1, \beta_2 = 0.9, 0.999$}~\cite{chen2020generative}& {$\beta_1, \beta_2 = 0.9, 0.999$} \\
Per GPU batch size &    12&12 \\
Drop out & 0.5 & 0.0\\
Drop path& 0.2 & 0.1 \\
Color jitter&   0.4&0.4 \\
Flip augmentation & \checkmark & \checkmark \\
Mixup~\cite{zhang2017mixup} & $\times$ & $\times$ \\
Cutmix~\cite{yun2019cutmix} & $\times$ & $\times$ \\
Random erasing~\cite{zhong2020random} & $\times$ & $\times$\\
Layer-wise learning rate decay~\cite{bao2021beit}&    0.75&0.75 \\
Learning rate schedule  & cosine decay~\cite{cosineannealing} & cosine decay\\
Warmup epochs & 5 & 5 \\
Training epochs &    100&100 \\
\bottomrule
\end{tabular}
}
\vspace{.2em}

\label{tab:baseline_noaug}
\end{table}
