# Supplementary material for: DEVIAS: Learning Disentangled Video Representations of Action and Scene
Source: arXiv:2312.00826 source file (2024-09-06)
Supplement: Supplementary file 5 [file supp_preamble.tex]

\usepackage{setspace}

\let\titleold\title
\let\instituteold\institute
\let\authorold\author
% \let\authorrunningold\authorrunning

\renewcommand{\title}[1]{\titleold{#1}\newcommand{\thetitle}{#1}}
\renewcommand{\institute}[1]{\instituteold{#1}\newcommand{\theinstitute}{#1}}
\renewcommand{\author}[1]{\authorold{#1}\newcommand{\theauthor}{#1}}
% \renewcommand{\authorrunning}[1]{\authorrunningold{#1}\newcommand{\theauthorrunning}{#1}}


\newcommand\maketitlesupplementary
   {\newpage
   {\centering \doublespacing 
    {\Large \textbf{\thetitle}} \\
    {\large \textbf{Supplementary Material} \\[-0.5ex]
    % {\normalsize ECCV 2024 Submission \#9270} \\
   }
   }
}

\newcommand{\maketitlesupplementaryfull}
   {
    \subtitle{Supplementary Material\vspace{-1em}}
    \titleold{\thetitle}
    \authorold{\theauthor}
    % \authorrunningold{\authorrunning}
    \instituteold{\theinstitute}
    \maketitle
   }

    
    % {\centering
    % \Large
    % \textbf{\thetitle}\\
    % \vspace{0.5em}
    % {\large \textbf{Supplementary Material}} \\
    %     \theinstitute
    % }
   

%   % Replace authors, institute, and running title with review placeholders
%   \let\maketitleold\maketitle
  % \renewcommand{\maketitle}{\author{Anonymous ECCV \eccv@year{} Submission}%
  %                           \titlerunning{ECCV \eccv@year{} Submission \#\eccv@ID}% 
  %                           \authorrunning{ECCV \eccv@year{} Submission \#\eccv@ID}% 
  %                           \institute{Paper ID \#\eccv@ID}%
  %                           \maketitleold}


% \makeatletter
% \ifeccv@review
%   % Display line numbers
%   \AtBeginDocument{%
%     \linenumbers
%     \linenomathpatch{equation}%
%     \linenomathpatchAMS{gather}%
%     \linenomathpatchAMS{multline}%
%     \linenomathpatchAMS{align}%
%     \linenomathpatchAMS{alignat}%
%     \linenomathpatchAMS{flalign}%
%   }

%   % Crop the page for review version
%   \RequirePackage[width=122mm,left=12mm,paperwidth=146mm,height=193mm,top=12mm,paperheight=217mm]{geometry}

%   % Replace authors, institute, and running title with review placeholders
%   \let\maketitleold\maketitle
%   \renewcommand{\maketitle}{\author{Anonymous ECCV \eccv@year{} Submission}%
%                             \titlerunning{ECCV \eccv@year{} Submission \#\eccv@ID}% 
%                             \authorrunning{ECCV \eccv@year{} Submission \#\eccv@ID}% 
%                             \institute{Paper ID \#\eccv@ID}%
%                             \maketitleold}
% \fi

% \makeatother
